# Supplementary material for: CodeCytos: AI-assisted spatial molecular imaging analysis via code-augmented agent action space
Source: arXiv:2606.00472 source file (2026-05-30)
Supplement: Supplementary file 1 [file supp.tex]

% \begin{landscape}

% \begingroup
% \setlength{\LTleft}{0pt plus 0fill}
% \setlength{\LTright}{0pt plus 0fill}
% \setlength{\tabcolsep}{0.2pt} % Reduce column spacing (default is 6pt)
% \tiny % Use tiny font for very wide tables

% \begin{longtable}{|l|cccc|cccc|cccc|cccc|cccc|cccc|}
% \caption{Comparison of models on selected metrics across datasets and shot settings (values rounded to two decimal places)}
% \label{tab:selected_metrics} \\
% \hline
% \textbf{Metric} & \multicolumn{4}{c|}{\textbf{Conventional LLM}} & \multicolumn{4}{c|}{\textbf{Conventional LLM with Zero-Shot CoT}} & \multicolumn{4}{c|}{\textbf{Conventional LLM with Few-Shot CoT}} & \multicolumn{4}{c|}{\textbf{CodeAct}} & \multicolumn{4}{c|}{\textbf{CodeAct + One Shot}} & \multicolumn{4}{c|}{\textbf{CodeAct + Few Shot}} \\
% \hline
% \textbf{Dataset} 
%  & \rotatebox{90}{\textcolor{blue!60!black}{Frontal\_Cortex}} & \rotatebox{90}{\textcolor{red!70!black}{NSCLC}} & \rotatebox{90}{\textcolor{violet}{Pancreas}} & \rotatebox{90}{\textcolor{orange!90!black}{Tonsil}}
%  & \rotatebox{90}{\textcolor{blue!60!black}{Frontal\_Cortex}} & \rotatebox{90}{\textcolor{red!70!black}{NSCLC}} & \rotatebox{90}{\textcolor{violet}{Pancreas}} & \rotatebox{90}{\textcolor{orange!90!black}{Tonsil}}
%  & \rotatebox{90}{\textcolor{blue!60!black}{Frontal\_Cortex}} & \rotatebox{90}{\textcolor{red!70!black}{NSCLC}} & \rotatebox{90}{\textcolor{violet}{Pancreas}} & \rotatebox{90}{\textcolor{orange!90!black}{Tonsil}}
%  & \rotatebox{90}{\textcolor{blue!60!black}{Frontal\_Cortex}} & \rotatebox{90}{\textcolor{red!70!black}{NSCLC}} & \rotatebox{90}{\textcolor{violet}{Pancreas}} & \rotatebox{90}{\textcolor{orange!90!black}{Tonsil}}
%  & \rotatebox{90}{\textcolor{blue!60!black}{Frontal\_Cortex}} & \rotatebox{90}{\textcolor{red!70!black}{NSCLC}} & \rotatebox{90}{\textcolor{violet}{Pancreas}} & \rotatebox{90}{\textcolor{orange!90!black}{Tonsil}}
%  & \rotatebox{90}{\textcolor{blue!60!black}{Frontal\_Cortex}} & \rotatebox{90}{\textcolor{red!70!black}{NSCLC}} & \rotatebox{90}{\textcolor{violet}{Pancreas}} & \rotatebox{90}{\textcolor{orange!90!black}{Tonsil}} \\
% \hline
% \endfirsthead

% \multicolumn{25}{c}%
% {{\tablename\ \thetable{} -- continued from previous page}} \\
% \hline
% \textbf{Metric} & \multicolumn{4}{c|}{\textbf{Conventional LLM}} & \multicolumn{4}{c|}{\textbf{CodeAct}} & \multicolumn{4}{c|}{\textbf{CodeAct + One Shot}} & \multicolumn{4}{c|}{\textbf{CodeAct + Few Shot}} \\
% \hline
% \textbf{Dataset} 
%  & \rotatebox{90}{\textcolor{blue!60!black}{Frontal\_Cortex}} & \rotatebox{90}{\textcolor{red!70!black}{NSCLC}} & \rotatebox{90}{\textcolor{violet}{Pancreas}} & \rotatebox{90}{\textcolor{orange!90!black}{Tonsil}}
%  & \rotatebox{90}{\textcolor{blue!60!black}{Frontal\_Cortex}} & \rotatebox{90}{\textcolor{red!70!black}{NSCLC}} & \rotatebox{90}{\textcolor{violet}{Pancreas}} & \rotatebox{90}{\textcolor{orange!90!black}{Tonsil}}
%  & \rotatebox{90}{\textcolor{blue!60!black}{Frontal\_Cortex}} & \rotatebox{90}{\textcolor{red!70!black}{NSCLC}} & \rotatebox{90}{\textcolor{violet}{Pancreas}} & \rotatebox{90}{\textcolor{orange!90!black}{Tonsil}}
%  & \rotatebox{90}{\textcolor{blue!60!black}{Frontal\_Cortex}} & \rotatebox{90}{\textcolor{red!70!black}{NSCLC}} & \rotatebox{90}{\textcolor{violet}{Pancreas}} & \rotatebox{90}{\textcolor{orange!90!black}{Tonsil}} \\
% \hline
% \endhead

% \hline
% \multicolumn{25}{|r|}{{Continued on next page}} \\
% \hline
% \endfoot

% \hline
% \endlastfoot

% \multicolumn{25}{|l|}{\textbf{Qwen 2.5 Coder}} \\
% \multicolumn{25}{|l|}{\textit{\quad Year: \hspace{2cm} Size: \hspace{2cm} Pretrain Data: }} \\
% \hline
% success\_rate & \cellcolor{blue!15}2.35 & \cellcolor{red!15}6.07 & \cellcolor{violet!15}4.02 & \cellcolor{orange!15}4.65 & 2.60 & 5.69 & 4.01 & 5.62 & 3.95 & 5.97 & 3.78 & 7.17 & 0.75 & 0.60 & 0.62 & 0.89 & 0.16 & 0.45 & 0.63 & 1.53 & \cellcolor{blue!45}36.61 & \cellcolor{red!45}54.28 & \cellcolor{violet!45}32.44 & \cellcolor{orange!45}47.65 \\
% {\tiny CI} & \cellcolor{blue!15}{\tiny [1.40, 3.39]} & \cellcolor{red!15}{\tiny [4.03, 8.43]} & \cellcolor{violet!15}{\tiny [2.67, 5.50]} & \cellcolor{orange!15}{\tiny [3.24, 6.17]} & {\tiny [1.51, 3.87]} & {\tiny [3.81, 7.84]} & {\tiny [2.59, 5.58]} & {\tiny [3.88, 7.51]} & {\tiny [2.45, 5.65]} & {\tiny [4.03, 8.21]} & {\tiny [2.52, 5.19]} & {\tiny [5.09, 9.48]} & {\tiny [0.33, 1.24]} & {\tiny [0.22, 1.12]} & {\tiny [0.24, 1.10]} & {\tiny [0.51, 1.34]} & {\tiny [0.00, 0.40]} & {\tiny [0.15, 0.82]} & {\tiny [0.16, 1.18]} & {\tiny [0.95, 2.16]} & \cellcolor{blue!45}{\tiny [30.87, 42.33]} & \cellcolor{red!45}{\tiny [49.10, 59.55]} & \cellcolor{violet!45}{\tiny [27.21, 37.51]} & \cellcolor{orange!45}{\tiny [41.97, 53.49]} \\
% \cline{1-25}
% pass@5       & \cellcolor{blue!15}10.52 & \cellcolor{red!15}19.62 & \cellcolor{violet!15}15.14 & \cellcolor{orange!15}18.33 & 10.53 & 19.30 & 14.18 & 20.51 & 14.66 & 20.34 & 14.85 & 23.22 & 3.72 & 2.80 & 3.16 & 4.45 & 0.80 & 2.26 & 2.69 & 7.40 & \cellcolor{blue!45}65.56 & \cellcolor{red!45}83.24 & \cellcolor{violet!45}57.22 & \cellcolor{orange!45}76.88 \\
% {\tiny CI} & \cellcolor{blue!15}{\tiny [6.72, 14.70]} & \cellcolor{red!15}{\tiny [14.40, 25.19]} & \cellcolor{violet!15}{\tiny [10.61, 20.17]} & \cellcolor{orange!15}{\tiny [13.63, 23.37]} & {\tiny [6.43, 15.18]} & {\tiny [14.29, 24.77]} & {\tiny [9.57, 19.14]} & {\tiny [15.49, 25.72]} & {\tiny [9.76, 19.87]} & {\tiny [15.06, 25.92]} & {\tiny [10.39, 19.73]} & {\tiny [17.63, 29.14]} & {\tiny [1.61, 6.14]} & {\tiny [1.12, 5.06]} & {\tiny [1.18, 5.50]} & {\tiny [2.23, 6.68]} & {\tiny [0.00, 2.02]} & {\tiny [0.75, 4.10]} & {\tiny [0.79, 5.00]} & {\tiny [4.66, 10.38]} & \cellcolor{blue!45}{\tiny [58.12, 72.77]} & \cellcolor{red!45}{\tiny [77.45, 88.69]} & \cellcolor{violet!45}{\tiny [49.96, 64.68]} & \cellcolor{orange!45}{\tiny [70.30, 82.97]} \\
% \cline{1-25}
% pass@10      & \cellcolor{blue!15}17.63 & \cellcolor{red!15}29.85 & \cellcolor{violet!15}20.15 & \cellcolor{orange!15}29.04 & 16.13 & 29.93 & 18.26 & 32.12 & 21.82 & 30.58 & 20.76 & 33.13 & 7.27 & 5.20 & 5.04 & 8.91 & 1.59 & 4.51 & 3.75 & 14.22 & \cellcolor{blue!45}73.45 & \cellcolor{red!45}87.26 & \cellcolor{violet!45}60.32 & \cellcolor{orange!45}82.52 \\
% {\tiny CI} & \cellcolor{blue!15}{\tiny [11.29, 24.21]} & \cellcolor{red!15}{\tiny [22.39, 38.06]} & \cellcolor{violet!15}{\tiny [13.84, 27.04]} & \cellcolor{orange!15}{\tiny [21.93, 36.48]} & {\tiny [9.68, 22.58]} & {\tiny [22.39, 38.06]} & {\tiny [12.58, 24.53]} & {\tiny [24.95, 39.81]} & {\tiny [14.52, 29.03]} & {\tiny [23.13, 38.81]} & {\tiny [14.47, 27.04]} & {\tiny [25.76, 40.86]} & {\tiny [3.23, 12.10]} & {\tiny [1.49, 8.96]} & {\tiny [1.89, 8.81]} & {\tiny [4.45, 13.36]} & {\tiny [0.00, 4.03]} & {\tiny [1.49, 8.21]} & {\tiny [1.26, 6.92]} & {\tiny [9.02, 19.55]} & \cellcolor{blue!45}{\tiny [65.32, 80.65]} & \cellcolor{red!45}{\tiny [81.34, 92.54]} & \cellcolor{violet!45}{\tiny [52.20, 67.92]} & \cellcolor{orange!45}{\tiny [75.90, 88.76]} \\
% \cline{1-25}
% pass@20      & \cellcolor{blue!15}17.81 & \cellcolor{red!15}29.89 & \cellcolor{violet!15}20.03 & \cellcolor{orange!15}32.01 & 16.15 & 29.87 & 18.28 & 35.82 & 21.77 & 30.63 & 20.80 & 35.96 & 7.29 & 5.19 & 5.01 & 10.70 & 1.61 & 4.43 & 3.75 & 16.77 & \cellcolor{blue!45}73.37 & \cellcolor{red!45}87.27 & \cellcolor{violet!45}60.41 & \cellcolor{orange!45}83.17 \\
% {\tiny CI} & \cellcolor{blue!15}{\tiny [11.29, 25.00]} & \cellcolor{red!15}{\tiny [22.39, 37.31]} & \cellcolor{violet!15}{\tiny [13.84, 26.42]} & \cellcolor{orange!15}{\tiny [24.43, 40.46]} & {\tiny [9.68, 22.58]} & {\tiny [22.39, 38.06]} & {\tiny [12.58, 24.53]} & {\tiny [27.48, 43.51]} & {\tiny [14.52, 29.03]} & {\tiny [23.13, 38.81]} & {\tiny [14.47, 27.04]} & {\tiny [28.24, 44.27]} & {\tiny [3.23, 12.10]} & {\tiny [1.49, 8.96]} & {\tiny [1.89, 8.81]} & {\tiny [5.34, 16.03]} & {\tiny [0.00, 4.03]} & {\tiny [1.49, 8.21]} & {\tiny [1.26, 6.92]} & {\tiny [10.69, 23.66]} & \cellcolor{blue!45}{\tiny [65.32, 80.65]} & \cellcolor{red!45}{\tiny [81.34, 92.54]} & \cellcolor{violet!45}{\tiny [52.83, 67.92]} & \cellcolor{orange!45}{\tiny [76.34, 89.31]} \\
% \cline{1-25}
% AUP@k        & \cellcolor{blue!15}0.11 & \cellcolor{red!15}0.20 & \cellcolor{violet!15}0.13 & \cellcolor{orange!15}0.21 & 0.11 & 0.20 & 0.13 & 0.23 & 0.15 & 0.20 & 0.13 & 0.25 & 0.04 & 0.03 & 0.03 & 0.06 & 0.01 & 0.02 & 0.02 & 0.09 & \cellcolor{blue!45}0.64 & \cellcolor{red!45}0.81 & \cellcolor{violet!45}0.53 & \cellcolor{orange!45}0.76 \\
% {\tiny CI} & \cellcolor{blue!15}{\tiny [0.07, 0.16]} & \cellcolor{red!15}{\tiny [0.15, 0.25]} & \cellcolor{violet!15}{\tiny [0.09, 0.18]} & \cellcolor{orange!15}{\tiny [0.15, 0.26]} & {\tiny [0.07, 0.15]} & {\tiny [0.15, 0.25]} & {\tiny [0.08, 0.17]} & {\tiny [0.18, 0.29]} & {\tiny [0.10, 0.20]} & {\tiny [0.15, 0.26]} & {\tiny [0.09, 0.18]} & {\tiny [0.19, 0.31]} & {\tiny [0.02, 0.07]} & {\tiny [0.01, 0.05]} & {\tiny [0.01, 0.05]} & {\tiny [0.03, 0.09]} & {\tiny [0.00, 0.02]} & {\tiny [0.01, 0.05]} & {\tiny [0.01, 0.05]} & {\tiny [0.06, 0.13]} & \cellcolor{blue!45}{\tiny [0.56, 0.71]} & \cellcolor{red!45}{\tiny [0.75, 0.86]} & \cellcolor{violet!45}{\tiny [0.47, 0.60]} & \cellcolor{orange!45}{\tiny [0.70, 0.82]} \\
% \hline
% \multicolumn{25}{|l|}{\textbf{Qwen 3 Coder}} \\
% \multicolumn{25}{|l|}{\textit{\quad Year: \hspace{2cm} Size: \hspace{2cm} Pretrain Data: }} \\
% \hline
% success\_rate & 1.61 & 1.94 & 1.26 & 1.65 & 1.00 & 2.39 & 0.50 & 1.70 & 1.42 & 2.17 & 1.18 & 2.47 & 24.90 & 36.04 & 17.62 & 24.68 & \cellcolor{blue!15}44.53 & \cellcolor{red!15}60.46 & \cellcolor{violet!15}33.67 & \cellcolor{orange!15}52.25 & \cellcolor{blue!45}48.67 & \cellcolor{red!45}63.10 & \cellcolor{violet!45}39.28 & \cellcolor{orange!45}58.55 \\
% {\tiny 95\% CI} & {\tiny [0.89, 2.50]} & {\tiny [0.90, 3.36]} & {\tiny [0.63, 2.04]} & {\tiny [0.76, 2.80]} & {\tiny [0.41, 1.76]} & {\tiny [1.19, 3.81]} & {\tiny [0.08, 1.00]} & {\tiny [0.70, 2.93]} & {\tiny [0.68, 2.26]} & {\tiny [1.19, 3.28]} & {\tiny [0.55, 1.89]} & {\tiny [1.34, 3.88]} & {\tiny [20.86, 29.07]} & {\tiny [31.42, 40.60]} & {\tiny [13.87, 21.51]} & {\tiny [20.99, 28.37]} & \cellcolor{blue!15}{\tiny [38.36, 50.54]} & \cellcolor{red!15}{\tiny [54.33, 66.34]} & \cellcolor{violet!15}{\tiny [28.25, 39.29]} & \cellcolor{orange!15}{\tiny [46.17, 58.04]} & \cellcolor{blue!45}{\tiny [42.58, 55.16]} & \cellcolor{red!45}{\tiny [56.86, 69.10]} & \cellcolor{violet!45}{\tiny [33.41, 45.20]} & \cellcolor{orange!45}{\tiny [52.48, 64.25]} \\
% \cline{1-25}
% pass@5       & 7.22 & 7.25 & 5.64 & 6.19 & 4.30 & 8.66 & 2.23 & 6.22 & 6.42 & 8.98 & 5.20 & 9.06 & 60.39 & 73.80 & 41.58 & 61.44 & \cellcolor{blue!15}71.61 & \cellcolor{red!15}82.35 & \cellcolor{violet!15}58.50 & \cellcolor{orange!15}78.30 & \cellcolor{blue!45}73.17 & \cellcolor{red!45}82.45 & \cellcolor{violet!45}60.18 & \cellcolor{orange!45}81.60 \\
% {\tiny 95\% CI} & {\tiny [4.08, 10.80]} & {\tiny [4.10, 10.88]} & {\tiny [2.92, 8.70]} & {\tiny [3.18, 9.50]} & {\tiny [1.70, 7.37]} & {\tiny [4.98, 12.75]} & {\tiny [0.39, 4.42]} & {\tiny [3.25, 9.62]} & {\tiny [3.36, 9.86]} & {\tiny [5.41, 12.88]} & {\tiny [2.53, 8.31]} & {\tiny [5.61, 12.90]} & {\tiny [53.34, 67.18]} & {\tiny [67.31, 79.87]} & {\tiny [34.73, 48.55]} & {\tiny [54.54, 67.94]} & \cellcolor{blue!15}{\tiny [64.05, 78.66]} & \cellcolor{red!15}{\tiny [76.47, 87.78]} & \cellcolor{violet!15}{\tiny [51.30, 65.51]} & \cellcolor{orange!15}{\tiny [72.02, 84.37]} & \cellcolor{blue!45}{\tiny [65.68, 80.13]} & \cellcolor{red!45}{\tiny [76.31, 88.14]} & \cellcolor{violet!45}{\tiny [52.96, 67.43]} & \cellcolor{orange!45}{\tiny [75.73, 87.12]} \\
% \cline{1-25}
% pass@10      & 12.86 & 12.68 & 8.14 & 10.12 & 7.34 & 13.40 & 3.16 & 10.06 & 11.30 & 14.94 & 7.56 & 15.29 & 74.18 & 83.51 & 46.57 & 72.92 & \cellcolor{blue!45}77.36 & \cellcolor{red!45}88.10 & \cellcolor{violet!15}62.79 & \cellcolor{orange!15}83.75 & \cellcolor{blue!45}77.32 & \cellcolor{red!15}85.81 & \cellcolor{violet!45}64.86 & \cellcolor{orange!45}87.12 \\
% {\tiny 95\% CI} & {\tiny [7.26, 19.35]} & {\tiny [7.46, 18.66]} & {\tiny [3.77, 12.58]} & {\tiny [5.44, 15.08]} & {\tiny [3.23, 12.10]} & {\tiny [8.21, 19.40]} & {\tiny [0.63, 6.29]} & {\tiny [5.34, 15.00]} & {\tiny [5.65, 16.94]} & {\tiny [8.96, 20.90]} & {\tiny [3.77, 11.95]} & {\tiny [9.92, 21.11]} & {\tiny [66.13, 81.45]} & {\tiny [76.87, 89.55]} & {\tiny [38.99, 54.09]} & {\tiny [65.43, 80.15]} & \cellcolor{blue!45}{\tiny [69.35, 84.68]} & \cellcolor{red!45}{\tiny [82.09, 93.28]} & \cellcolor{violet!15}{\tiny [55.35, 70.44]} & \cellcolor{orange!15}{\tiny [77.56, 89.46]} & \cellcolor{blue!45}{\tiny [70.16, 83.87]} & \cellcolor{red!15}{\tiny [79.85, 91.79]} & \cellcolor{violet!45}{\tiny [57.23, 72.33]} & \cellcolor{orange!45}{\tiny [81.48, 92.44]} \\
% \cline{1-25}
% pass@20      & 12.93 & 12.71 & 8.17 & 11.45 & 7.22 & 13.43 & 3.16 & 11.46 & 11.34 & 14.93 & 7.56 & 17.51 & 74.27 & 83.60 & 46.52 & 74.72 & \cellcolor{blue!45}77.39 & \cellcolor{red!45}88.05 & \cellcolor{violet!15}62.93 & \cellcolor{orange!15}84.75 & \cellcolor{blue!45}77.41 & \cellcolor{red!15}85.83 & \cellcolor{violet!45}64.76 & \cellcolor{orange!45}88.53 \\
% {\tiny 95\% CI} & {\tiny [7.26, 18.55]} & {\tiny [7.46, 18.66]} & {\tiny [4.40, 12.58]} & {\tiny [6.11, 17.56]} & {\tiny [3.23, 12.10]} & {\tiny [8.21, 19.40]} & {\tiny [0.63, 6.29]} & {\tiny [6.11, 17.56]} & {\tiny [6.43, 16.94]} & {\tiny [8.96, 20.90]} & {\tiny [3.77, 11.95]} & {\tiny [11.45, 24.43]} & {\tiny [66.13, 81.45]} & {\tiny [76.87, 89.55]} & {\tiny [38.99, 54.09]} & {\tiny [67.18, 81.68]} & \cellcolor{blue!45}{\tiny [70.16, 84.68]} & \cellcolor{red!45}{\tiny [82.09, 93.28]} & \cellcolor{violet!15}{\tiny [55.35, 70.44]} & \cellcolor{orange!15}{\tiny [78.63, 90.84]} & \cellcolor{blue!45}{\tiny [69.35, 84.68]} & \cellcolor{red!15}{\tiny [79.85, 91.79]} & \cellcolor{violet!45}{\tiny [57.23, 71.70]} & \cellcolor{orange!45}{\tiny [82.44, 93.89]} \\
% \cline{1-25}
% AUP@k        & 0.08 & 0.08 & 0.05 & 0.07 & 0.05 & 0.09 & 0.02 & 0.07 & 0.07 & 0.09 & 0.05 & 0.11 & 0.59 & 0.71 & 0.38 & 0.62 & \cellcolor{blue!15}0.70 & \cellcolor{red!45}0.81 & \cellcolor{violet!15}0.55 & \cellcolor{orange!15}0.78 & \cellcolor{blue!45}0.71 & \cellcolor{red!45}0.81 & \cellcolor{violet!45}0.57 & \cellcolor{orange!45}0.82 \\
% {\tiny 95\% CI} & {\tiny [0.043, 0.115]} & {\tiny [0.042, 0.114]} & {\tiny [0.025, 0.078]} & {\tiny [0.039, 0.110]} & {\tiny [0.018, 0.075]} & {\tiny [0.052, 0.129]} & {\tiny [0.004, 0.039]} & {\tiny [0.039, 0.108]} & {\tiny [0.036, 0.105]} & {\tiny [0.057, 0.133]} & {\tiny [0.023, 0.075]} & {\tiny [0.068, 0.150]} & {\tiny [0.520, 0.650]} & {\tiny [0.650, 0.767]} & {\tiny [0.314, 0.440]} & {\tiny [0.551, 0.679]} & \cellcolor{blue!15}{\tiny [0.626, 0.764]} & \cellcolor{red!45}{\tiny [0.754, 0.865]} & \cellcolor{violet!15}{\tiny [0.480, 0.615]} & \cellcolor{orange!15}{\tiny [0.718, 0.837]} & \cellcolor{blue!45}{\tiny [0.643, 0.778]} & \cellcolor{red!45}{\tiny [0.750, 0.865]} & \cellcolor{violet!45}{\tiny [0.504, 0.642]} & \cellcolor{orange!45}{\tiny [0.758, 0.868]} \\
% \hline
% \multicolumn{25}{|l|}{\textbf{Facebook CWM}} \\
% \multicolumn{25}{|l|}{\textit{\quad Year: \hspace{2cm} Size: \hspace{2cm} Pretrain Data: }} \\
% \hline
% success\_rate & 0.64 & 2.45 & 1.19 & 2.05 & 0.97 & 1.72 & 0.71 & 1.34 & 0.48 & 2.01 & 0.39 & 1.21 & 18.13 & 26.02 & 14.49 & 29.06 & \cellcolor{blue!15}29.80 & \cellcolor{red!15}41.49 & \cellcolor{violet!15}23.65 & \cellcolor{orange!15}42.62 & \cellcolor{blue!45}32.91 & \cellcolor{red!45}46.61 & \cellcolor{violet!45}27.10 & \cellcolor{orange!45}44.44 \\
% {\tiny 95\% CI} & {\tiny [0.24, 1.21]} & {\tiny [1.42, 3.73]} & {\tiny [0.55, 1.97]} & {\tiny [0.95, 3.63]} & {\tiny [0.40, 1.61]} & {\tiny [0.60, 3.21]} & {\tiny [0.24, 1.26]} & {\tiny [0.51, 2.42]} & {\tiny [0.16, 0.89]} & {\tiny [0.75, 3.81]} & {\tiny [0.08, 0.79]} & {\tiny [0.57, 2.04]} & {\tiny [14.98, 21.51]} & {\tiny [22.76, 29.18]} & {\tiny [11.64, 17.50]} & {\tiny [25.28, 32.97]} & \cellcolor{blue!15}{\tiny [25.05, 34.59]} & \cellcolor{red!15}{\tiny [36.94, 46.12]} & \cellcolor{violet!15}{\tiny [19.42, 28.07]} & \cellcolor{orange!15}{\tiny [37.36, 47.84]} & \cellcolor{blue!45}{\tiny [27.96, 38.22]} & \cellcolor{red!45}{\tiny [41.42, 51.64]} & \cellcolor{violet!45}{\tiny [22.54, 31.84]} & \cellcolor{orange!45}{\tiny [39.04, 49.67]} \\
% \cline{1-25}
% pass@5       & 3.08 & 9.89 & 5.20 & 7.54 & 2.80 & 3.91 & 2.06 & 3.39 & 1.45 & 4.33 & 1.18 & 3.28 & 53.53 & 67.63 & 43.00 & 68.72 & \cellcolor{blue!15}66.65 & \cellcolor{red!15}78.34 & \cellcolor{violet!15}50.49 & \cellcolor{orange!15}76.26 & \cellcolor{blue!45}67.67 & \cellcolor{red!45}78.07 & \cellcolor{violet!45}53.18 & \cellcolor{orange!45}77.15 \\
% {\tiny 95\% CI} & {\tiny [1.21, 5.47]} & {\tiny [6.16, 13.89]} & {\tiny [2.53, 8.14]} & {\tiny [4.45, 10.93]} & {\tiny [1.61, 4.49]} & {\tiny [3.21, 5.60]} & {\tiny [1.26, 3.28]} & {\tiny [2.31, 4.98]} & {\tiny [0.89, 2.44]} & {\tiny [3.81, 6.18]} & {\tiny [0.79, 1.97]} & {\tiny [2.04, 5.08]} & {\tiny [46.17, 60.62]} & {\tiny [61.04, 74.11]} & {\tiny [36.17, 49.84]} & {\tiny [62.31, 74.78]} & \cellcolor{blue!15}{\tiny [59.40, 73.62]} & \cellcolor{red!15}{\tiny [71.98, 84.08]} & \cellcolor{violet!15}{\tiny [43.36, 57.27]} & \cellcolor{orange!15}{\tiny [69.58, 82.31]} & \cellcolor{blue!45}{\tiny [60.39, 74.77]} & \cellcolor{red!45}{\tiny [71.64, 84.07]} & \cellcolor{violet!45}{\tiny [45.42, 60.86]} & \cellcolor{orange!45}{\tiny [70.77, 83.27]} \\
% \cline{1-25}
% pass@10      & 5.71 & 16.44 & 7.58 & 13.24 & 4.48 & 5.60 & 3.31 & 4.98 & 2.42 & 6.18 & 1.97 & 5.08 & 65.27 & 78.28 & 51.02 & 80.87 & \cellcolor{blue!15}75.07 & \cellcolor{red!15}85.03 & \cellcolor{violet!15}57.16 & \cellcolor{orange!15}82.71 & \cellcolor{blue!45}75.01 & \cellcolor{red!45}83.60 & \cellcolor{violet!45}54.69 & \cellcolor{orange!45}82.89 \\
% {\tiny 95\% CI} & {\tiny [2.42, 9.68]} & {\tiny [10.45, 23.13]} & {\tiny [3.77, 11.95]} & {\tiny [8.00, 18.69]} & {\tiny [2.02, 7.48]} & {\tiny [5.22, 8.58]} & {\tiny [1.18, 5.67]} & {\tiny [3.94, 8.14]} & {\tiny [0.81, 4.44]} & {\tiny [5.22, 9.70]} & {\tiny [0.39, 3.93]} & {\tiny [5.09, 7.93]} & {\tiny [56.45, 73.39]} & {\tiny [70.90, 85.07]} & {\tiny [43.40, 59.12]} & {\tiny [74.37, 86.77]} & \cellcolor{blue!15}{\tiny [66.94, 82.26]} & \cellcolor{red!15}{\tiny [78.36, 91.04]} & \cellcolor{violet!15}{\tiny [49.69, 64.78]} & \cellcolor{orange!15}{\tiny [75.79, 88.71]} & \cellcolor{blue!45}{\tiny [66.94, 82.26]} & \cellcolor{red!45}{\tiny [76.87, 89.55]} & \cellcolor{violet!45}{\tiny [47.17, 62.26]} & \cellcolor{orange!45}{\tiny [76.12, 89.08]} \\
% \cline{1-25}
% pass@20      & 5.66 & 16.42 & 7.57 & 15.34 & 8.06 & 9.70 & 5.03 & 9.16 & 4.84 & 10.45 & 3.14 & 10.69 & 65.25 & 78.44 & 51.03 & 83.13 & \cellcolor{blue!15}74.95 & \cellcolor{red!15}85.14 & \cellcolor{violet!15}57.33 & \cellcolor{orange!15}83.23 & \cellcolor{blue!45}75.02 & \cellcolor{red!45}83.58 & \cellcolor{violet!45}54.70 & \cellcolor{orange!45}83.15 \\
% {\tiny 95\% CI} & {\tiny [1.61, 9.68]} & {\tiny [10.45, 23.13]} & {\tiny [3.77, 11.95]} & {\tiny [9.90, 21.37]} & {\tiny [3.23, 12.90]} & {\tiny [5.22, 14.93]} & {\tiny [1.89, 8.81]} & {\tiny [5.34, 14.50]} & {\tiny [1.61, 8.87]} & {\tiny [5.22, 15.67]} & {\tiny [0.63, 6.29]} & {\tiny [5.34, 16.03]} & {\tiny [57.26, 73.39]} & {\tiny [71.64, 85.07]} & {\tiny [43.40, 59.12]} & {\tiny [76.34, 89.31]} & \cellcolor{blue!15}{\tiny [66.94, 82.26]} & \cellcolor{red!15}{\tiny [79.10, 91.04]} & \cellcolor{violet!15}{\tiny [49.69, 64.78]} & \cellcolor{orange!15}{\tiny [76.34, 89.31]} & \cellcolor{blue!45}{\tiny [66.94, 82.26]} & \cellcolor{red!45}{\tiny [76.87, 89.55]} & \cellcolor{violet!45}{\tiny [47.15, 62.26]} & \cellcolor{orange!45}{\tiny [76.34, 89.31]} \\
% \cline{1-25}
% AUP@k        & 0.03 & 0.10 & 0.05 & 0.09 & 0.05 & 0.06 & 0.03 & 0.06 & 0.03 & 0.07 & 0.02 & 0.06 & 0.51 & 0.64 & 0.38 & 0.69 & \cellcolor{blue!15}0.64 & \cellcolor{red!15}0.75 & \cellcolor{violet!15}0.46 & \cellcolor{orange!15}0.75 & \cellcolor{blue!45}0.65 & \cellcolor{red!45}0.76 & \cellcolor{violet!45}0.49 & \cellcolor{orange!45}0.76 \\
% {\tiny 95\% CI} & {\tiny [0.013, 0.058]} & {\tiny [0.065, 0.144]} & {\tiny [0.023, 0.073]} & {\tiny [0.055, 0.130]} & {\tiny [0.021, 0.079]} & {\tiny [0.033, 0.092]} & {\tiny [0.011, 0.051]} & {\tiny [0.028, 0.091]} & {\tiny [0.009, 0.049]} & {\tiny [0.033, 0.101]} & {\tiny [0.004, 0.035]} & {\tiny [0.033, 0.096]} & {\tiny [0.445, 0.579]} & {\tiny [0.579, 0.701]} & {\tiny [0.321, 0.438]} & {\tiny [0.630, 0.746]} & \cellcolor{blue!15}{\tiny [0.567, 0.702]} & \cellcolor{red!15}{\tiny [0.694, 0.806]} & \cellcolor{violet!15}{\tiny [0.395, 0.526]} & \cellcolor{orange!15}{\tiny [0.687, 0.810]} & \cellcolor{blue!45}{\tiny [0.574, 0.713]} & \cellcolor{red!45}{\tiny [0.693, 0.815]} & \cellcolor{violet!45}{\tiny [0.418, 0.557]} & \cellcolor{orange!45}{\tiny [0.698, 0.817]} \\
% \hline
% \multicolumn{25}{|l|}{\textbf{Mistral/Devstral-Small}} \\
% \multicolumn{25}{|l|}{\textit{\quad Year: \hspace{2cm} Size: \hspace{2cm} Pretrain Data: }} \\
% \hline
% success\_rate & \cellcolor{blue!15}1.86 & \cellcolor{red!15}4.03 & \cellcolor{violet!15}2.44 & \cellcolor{orange!15}2.74 & 1.38 & 3.36 & 2.52 & 3.60 & 0.89 & 3.13 & 1.89 & 3.03 & 0.24 & 1.55 & 0.39 & 0.95 & 0.89 & 1.91 & 0.55 & 1.34 & \cellcolor{blue!45}34.80 & \cellcolor{red!45}52.93 & \cellcolor{violet!45}29.22 & \cellcolor{orange!45}45.24 \\
% {\tiny 95\% CI} & \cellcolor{blue!15}{\tiny [1.01, 2.85]} & \cellcolor{red!15}{\tiny [2.39, 6.04]} & \cellcolor{violet!15}{\tiny [1.23, 3.86]} & \cellcolor{orange!15}{\tiny [1.64, 4.06]} & {\tiny [0.73, 2.04]} & {\tiny [1.94, 5.07]} & {\tiny [1.47, 3.67]} & {\tiny [2.17, 5.30]} & {\tiny [0.32, 1.62]} & {\tiny [1.57, 5.07]} & {\tiny [1.03, 2.84]} & {\tiny [1.76, 4.43]} & {\tiny [0.00, 0.56]} & {\tiny [0.37, 3.28]} & {\tiny [0.00, 0.94]} & {\tiny [0.19, 2.16]} & {\tiny [0.41, 1.45]} & {\tiny [0.61, 3.76]} & {\tiny [0.16, 0.94]} & {\tiny [0.38, 2.80]} & \cellcolor{blue!45}{\tiny [29.16, 40.29]} & \cellcolor{red!45}{\tiny [47.11, 58.40]} & \cellcolor{violet!45}{\tiny [24.63, 33.92]} & \cellcolor{orange!45}{\tiny [39.48, 51.16]} \\
% \cline{1-25}
% pass@5       & \cellcolor{blue!15}8.04 & \cellcolor{red!15}14.04 & \cellcolor{violet!15}7.98 & \cellcolor{orange!15}11.07 & 4.06 & 8.33 & 6.81 & 8.96 & 2.45 & 6.97 & 5.15 & 7.80 & 1.21 & 3.93 & 1.42 & 2.99 & 4.42 & 5.80 & 2.77 & 4.26 & \cellcolor{blue!45}66.12 & \cellcolor{red!45}81.55 & \cellcolor{violet!45}59.71 & \cellcolor{orange!45}76.85 \\
% {\tiny 95\% CI} & \cellcolor{blue!15}{\tiny [4.35, 12.05]} & \cellcolor{red!15}{\tiny [9.56, 18.88]} & \cellcolor{violet!15}{\tiny [4.26, 12.16]} & \cellcolor{orange!15}{\tiny [7.51, 14.98]} & {\tiny [3.63, 9.90]} & {\tiny [6.42, 16.92]} & {\tiny [6.42, 14.40]} & {\tiny [8.92, 17.69]} & {\tiny [1.21, 6.61]} & {\tiny [3.77, 14.28]} & {\tiny [2.84, 11.88]} & {\tiny [4.43, 15.70]} & {\tiny [0.00, 2.82]} & {\tiny [1.49, 6.92]} & {\tiny [0.00, 3.20]} & {\tiny [1.08, 5.34]} & {\tiny [2.02, 7.26]} & {\tiny [3.03, 9.12]} & {\tiny [0.79, 4.72]} & {\tiny [1.91, 6.93]} & \cellcolor{blue!45}{\tiny [58.75, 73.19]} & \cellcolor{red!45}{\tiny [75.57, 86.92]} & \cellcolor{violet!45}{\tiny [52.79, 66.47]} & \cellcolor{orange!45}{\tiny [70.48, 83.01]} \\
% \cline{1-25}
% pass@10      & \cellcolor{blue!15}12.88 & \cellcolor{red!15}22.42 & \cellcolor{violet!15}9.43 & \cellcolor{orange!15}19.49 & 6.68 & 12.27 & 10.25 & 13.00 & 3.79 & 10.10 & 7.94 & 11.59 & 2.44 & 6.03 & 1.90 & 5.27 & 8.80 & 9.68 & 4.37 & 7.78 & \cellcolor{blue!45}74.12 & \cellcolor{red!45}86.56 & \cellcolor{violet!45}66.69 & \cellcolor{orange!45}83.62 \\
% {\tiny 95\% CI} & \cellcolor{blue!15}{\tiny [7.26, 19.35]} & \cellcolor{red!15}{\tiny [15.67, 29.85]} & \cellcolor{violet!15}{\tiny [5.03, 14.47]} & \cellcolor{orange!15}{\tiny [13.16, 26.28]} & {\tiny [7.26, 19.35]} & {\tiny [13.43, 26.88]} & {\tiny [8.81, 19.50]} & {\tiny [13.94, 27.26]} & {\tiny [1.21, 11.29]} & {\tiny [6.22, 23.13]} & {\tiny [4.53, 15.72]} & {\tiny [7.77, 25.83]} & {\tiny [0.00, 5.65]} & {\tiny [2.24, 10.45]} & {\tiny [0.00, 4.40]} & {\tiny [1.91, 9.03]} & {\tiny [4.03, 14.52]} & {\tiny [5.22, 14.93]} & {\tiny [1.26, 7.55]} & {\tiny [3.82, 12.21]} & \cellcolor{blue!45}{\tiny [66.13, 81.45]} & \cellcolor{red!45}{\tiny [80.60, 91.79]} & \cellcolor{violet!45}{\tiny [59.12, 74.21]} & \cellcolor{orange!45}{\tiny [77.12, 89.51]} \\
% \cline{1-25}
% pass@20      & \cellcolor{blue!15}12.86 & \cellcolor{red!15}22.42 & \cellcolor{violet!15}9.41 & \cellcolor{orange!15}21.43 & 12.90 & 20.15 & 13.84 & 20.54 & 6.45 & 16.42 & 10.69 & 19.45 & 2.40 & 5.97 & 1.89 & 6.16 & 8.81 & 9.73 & 4.42 & 9.10 & \cellcolor{blue!45}74.25 & \cellcolor{red!45}86.53 & \cellcolor{violet!45}66.62 & \cellcolor{orange!45}84.75 \\
% {\tiny 95\% CI} & \cellcolor{blue!15}{\tiny [7.26, 19.35]} & \cellcolor{red!15}{\tiny [15.67, 29.85]} & \cellcolor{violet!15}{\tiny [5.03, 14.47]} & \cellcolor{orange!15}{\tiny [14.50, 29.01]} & {\tiny [7.26, 19.35]} & {\tiny [14.18, 26.87]} & {\tiny [8.18, 19.50]} & {\tiny [15.27, 29.01]} & {\tiny [2.42, 11.29]} & {\tiny [10.45, 23.13]} & {\tiny [6.29, 15.72]} & {\tiny [13.31, 28.24]} & {\tiny [0.00, 5.65]} & {\tiny [2.24, 10.45]} & {\tiny [0.00, 4.40]} & {\tiny [2.29, 10.69]} & {\tiny [4.03, 14.52]} & {\tiny [5.22, 14.93]} & {\tiny [1.26, 7.55]} & {\tiny [4.58, 14.50]} & \cellcolor{blue!45}{\tiny [66.13, 81.45]} & \cellcolor{red!45}{\tiny [80.60, 91.79]} & \cellcolor{violet!45}{\tiny [59.12, 73.58]} & \cellcolor{orange!45}{\tiny [78.63, 90.84]} \\
% \cline{1-25}
% AUP@k        & \cellcolor{blue!15}0.08 & \cellcolor{red!15}0.14 & \cellcolor{violet!15}0.07 & \cellcolor{orange!15}0.13 & 0.07 & 0.13 & 0.09 & 0.15 & 0.04 & 0.10 & 0.07 & 0.14 & 0.01 & 0.04 & 0.01 & 0.04 & 0.05 & 0.06 & 0.02 & 0.05 & \cellcolor{blue!45}0.64 & \cellcolor{red!45}0.80 & \cellcolor{violet!45}0.55 & \cellcolor{orange!45}0.76 \\
% {\tiny 95\% CI} & \cellcolor{blue!15}{\tiny [0.05, 0.12]} & \cellcolor{red!15}{\tiny [0.10, 0.19]} & \cellcolor{violet!15}{\tiny [0.04, 0.11]} & \cellcolor{orange!15}{\tiny [0.09, 0.18]} & {\tiny [0.04, 0.11]} & {\tiny [0.08, 0.17]} & {\tiny [0.06, 0.13]} & {\tiny [0.10, 0.20]} & {\tiny [0.01, 0.07]} & {\tiny [0.06, 0.15]} & {\tiny [0.04, 0.10]} & {\tiny [0.09, 0.18]} & {\tiny [0.00, 0.03]} & {\tiny [0.02, 0.07]} & {\tiny [0.00, 0.03]} & {\tiny [0.01, 0.06]} & {\tiny [0.02, 0.08]} & {\tiny [0.03, 0.10]} & {\tiny [0.01, 0.04]} & {\tiny [0.02, 0.08]} & \cellcolor{blue!45}{\tiny [0.57, 0.71]} & \cellcolor{red!45}{\tiny [0.74, 0.85]} & \cellcolor{violet!45}{\tiny [0.48, 0.61]} & \cellcolor{orange!45}{\tiny [0.70, 0.82]} \\
% \hline
% \multicolumn{25}{|l|}{\textbf{Moonshot Kimi Linear 48B}} \\
% \multicolumn{25}{|l|}{\textit{\quad Year: \hspace{2cm} Size: 48B \hspace{2cm} Pretrain Data: }} \\
% \hline
% success\_rate & 0.56 & 1.64 & 0.16 & 0.95 & 0.81 & 1.34 & 0.71 & 1.08 & 0.65 & 2.09 & 0.79 & 1.34 & 2.18 & 3.66 & 2.52 & 2.99 & \cellcolor{blue!15}3.63 & \cellcolor{red!15}8.04 & \cellcolor{violet!15}4.17 & \cellcolor{orange!15}7.82 & \cellcolor{blue!45}17.86 & \cellcolor{red!45}21.21 & \cellcolor{violet!45}15.64 & \cellcolor{orange!45}21.44 \\
% {\tiny 95\% CI} & {\tiny [0.16, 1.13]} & {\tiny [0.67, 2.84]} & {\tiny [0.00, 0.39]} & {\tiny [0.25, 2.10]} & {\tiny [0.24, 1.45]} & {\tiny [0.67, 2.16]} & {\tiny [0.24, 1.26]} & {\tiny [0.38, 1.91]} & {\tiny [0.24, 1.13]} & {\tiny [1.12, 3.13]} & {\tiny [0.31, 1.37]} & {\tiny [0.64, 2.18]} & {\tiny [1.45, 3.06]} & {\tiny [2.31, 5.30]} & {\tiny [1.57, 3.54]} & {\tiny [1.97, 4.26]} & \cellcolor{blue!15}{\tiny [2.50, 4.92]} & \cellcolor{red!15}{\tiny [6.29, 9.89]} & \cellcolor{violet!15}{\tiny [2.99, 5.50]} & \cellcolor{orange!15}{\tiny [6.11, 9.61]} & \cellcolor{blue!45}{\tiny [14.67, 21.18]} & \cellcolor{red!45}{\tiny [18.20, 24.27]} & \cellcolor{violet!45}{\tiny [12.89, 18.40]} & \cellcolor{orange!45}{\tiny [18.07, 24.94]} \\
% \cline{1-25}
% pass@5       & 2.50 & 6.05 & 0.80 & 3.31 & 2.26 & 3.74 & 2.06 & 2.64 & 1.94 & 5.70 & 2.36 & 3.56 & 10.35 & 13.76 & 10.89 & 12.94 & \cellcolor{blue!15}15.77 & \cellcolor{red!15}31.34 & \cellcolor{violet!15}17.58 & \cellcolor{orange!15}30.23 & \cellcolor{blue!45}51.28 & \cellcolor{red!45}60.89 & \cellcolor{violet!45}46.73 & \cellcolor{orange!45}57.74 \\
% {\tiny 95\% CI} & {\tiny [0.63, 4.93]} & {\tiny [2.99, 9.56]} & {\tiny [0.00, 1.97]} & {\tiny [1.27, 5.66]} & {\tiny [1.21, 3.50]} & {\tiny [2.16, 5.78]} & {\tiny [1.18, 3.30]} & {\tiny [1.81, 3.82]} & {\tiny [1.13, 3.25]} & {\tiny [3.13, 8.74]} & {\tiny [1.28, 3.93]} & {\tiny [2.18, 5.53]} & {\tiny [6.68, 14.38]} & {\tiny [9.41, 18.47]} & {\tiny [7.02, 14.94]} & {\tiny [9.31, 16.91]} & \cellcolor{blue!15}{\tiny [11.16, 20.34]} & \cellcolor{red!15}{\tiny [25.50, 37.28]} & \cellcolor{violet!15}{\tiny [12.80, 22.46]} & \cellcolor{orange!15}{\tiny [24.82, 35.70]} & \cellcolor{blue!45}{\tiny [43.98, 58.49]} & \cellcolor{red!45}{\tiny [54.36, 67.40]} & \cellcolor{violet!45}{\tiny [40.32, 53.23]} & \cellcolor{orange!45}{\tiny [51.54, 63.89]} \\
% \cline{1-25}
% pass@10      & 4.02 & 9.75 & 1.26 & 5.81 & 3.49 & 5.78 & 3.31 & 3.94 & 3.23 & 8.75 & 3.93 & 5.53 & 19.35 & 23.13 & 15.72 & 24.02 & \cellcolor{blue!15}27.42 & \cellcolor{red!15}47.76 & \cellcolor{violet!15}25.16 & \cellcolor{orange!15}47.21 & \cellcolor{blue!45}65.32 & \cellcolor{red!45}75.37 & \cellcolor{violet!45}56.60 & \cellcolor{orange!45}73.54 \\
% {\tiny 95\% CI} & {\tiny [0.81, 8.06]} & {\tiny [5.22, 14.93]} & {\tiny [0.00, 3.14]} & {\tiny [2.54, 9.80]} & {\tiny [1.61, 5.63]} & {\tiny [2.86, 9.73]} & {\tiny [1.89, 5.01]} & {\tiny [3.18, 6.49]} & {\tiny [1.21, 5.65]} & {\tiny [5.27, 12.52]} & {\tiny [1.97, 6.68]} & {\tiny [3.18, 8.51]} & {\tiny [12.90, 26.61]} & {\tiny [16.42, 30.60]} & {\tiny [10.69, 21.38]} & {\tiny [17.79, 30.99]} & \cellcolor{blue!15}{\tiny [20.16, 35.48]} & \cellcolor{red!15}{\tiny [39.55, 55.97]} & \cellcolor{violet!15}{\tiny [18.24, 32.08]} & \cellcolor{orange!15}{\tiny [39.09, 54.88]} & \cellcolor{blue!45}{\tiny [57.26, 73.39]} & \cellcolor{red!45}{\tiny [67.91, 82.09]} & \cellcolor{violet!45}{\tiny [49.04, 64.15]} & \cellcolor{orange!45}{\tiny [66.59, 80.28]} \\
% \cline{1-25}
% pass@20      & 4.01 & 9.75 & 1.25 & 6.86 & 5.65 & 9.70 & 5.03 & 7.12 & 6.45 & 14.93 & 6.29 & 10.31 & 19.35 & 23.13 & 15.72 & 28.24 & \cellcolor{blue!15}27.42 & \cellcolor{red!15}47.76 & \cellcolor{violet!15}25.16 & \cellcolor{orange!15}51.91 & \cellcolor{blue!45}65.32 & \cellcolor{red!45}75.37 & \cellcolor{violet!45}56.60 & \cellcolor{orange!45}77.10 \\
% {\tiny 95\% CI} & {\tiny [0.81, 8.06]} & {\tiny [5.22, 14.93]} & {\tiny [0.00, 3.14]} & {\tiny [3.05, 11.45]} & {\tiny [2.42, 9.68]} & {\tiny [5.22, 14.93]} & {\tiny [2.52, 8.81]} & {\tiny [5.73, 11.29]} & {\tiny [2.42, 11.29]} & {\tiny [8.96, 20.90]} & {\tiny [3.14, 10.06]} & {\tiny [6.87, 15.27]} & {\tiny [12.90, 26.61]} & {\tiny [16.42, 30.60]} & {\tiny [10.06, 21.38]} & {\tiny [20.61, 35.88]} & \cellcolor{blue!15}{\tiny [19.35, 35.48]} & \cellcolor{red!15}{\tiny [38.81, 55.97]} & \cellcolor{violet!15}{\tiny [18.87, 32.08]} & \cellcolor{orange!15}{\tiny [43.51, 60.31]} & \cellcolor{blue!45}{\tiny [56.45, 73.39]} & \cellcolor{red!45}{\tiny [67.91, 82.84]} & \cellcolor{violet!45}{\tiny [49.06, 64.15]} & \cellcolor{orange!45}{\tiny [69.47, 83.97]} \\
% \cline{1-25}
% AUP@k        & 0.03 & 0.06 & 0.01 & 0.04 & 0.04 & 0.06 & 0.03 & 0.05 & 0.04 & 0.09 & 0.04 & 0.07 & 0.11 & 0.14 & 0.10 & 0.16 & \cellcolor{blue!15}0.17 & \cellcolor{red!15}0.32 & \cellcolor{violet!15}0.16 & \cellcolor{orange!15}0.34 & \cellcolor{blue!45}0.50 & \cellcolor{red!45}0.59 & \cellcolor{violet!45}0.42 & \cellcolor{orange!45}0.60 \\
% {\tiny 95\% CI} & {\tiny [0.00, 0.05]} & {\tiny [0.03, 0.10]} & {\tiny [0.00, 0.02]} & {\tiny [0.02, 0.07]} & {\tiny [0.01, 0.06]} & {\tiny [0.03, 0.09]} & {\tiny [0.01, 0.05]} & {\tiny [0.02, 0.08]} & {\tiny [0.01, 0.06]} & {\tiny [0.05, 0.13]} & {\tiny [0.02, 0.06]} & {\tiny [0.04, 0.10]} & {\tiny [0.07, 0.15]} & {\tiny [0.10, 0.19]} & {\tiny [0.06, 0.13]} & {\tiny [0.12, 0.21]} & \cellcolor{blue!15}{\tiny [0.12, 0.22]} & \cellcolor{red!15}{\tiny [0.26, 0.38]} & \cellcolor{violet!15}{\tiny [0.12, 0.20]} & \cellcolor{orange!15}{\tiny [0.29, 0.40]} & \cellcolor{blue!45}{\tiny [0.43, 0.56]} & \cellcolor{red!45}{\tiny [0.52, 0.65]} & \cellcolor{violet!45}{\tiny [0.36, 0.48]} & \cellcolor{orange!45}{\tiny [0.54, 0.66]} \\
% \hline
% \multicolumn{25}{|l|}{\textbf{GLM-4.5 Air}} \\
% \multicolumn{25}{|l|}{\textit{\quad Year: \hspace{2cm} Size: \hspace{2cm} Pretrain Data: }} \\
% \hline
% success\_rate & 0.08 & 0.45 & 0.08 & 0.83 & 0.16 & 0.45 & 0.16 & 0.95 & 0.32 & 0.45 & 0.24 & 1.21 & 21.35 & 20.83 & 13.45 & 17.87 & \cellcolor{blue!15}38.37 & \cellcolor{red!15}51.39 & \cellcolor{violet!15}33.28 & \cellcolor{orange!15}43.24 & \cellcolor{blue!45}50.00 & \cellcolor{red!45}61.55 & \cellcolor{violet!45}43.66 & \cellcolor{orange!45}61.61 \\
% {\tiny CI} & {\tiny [0.00, 0.24]} & {\tiny [0.07, 1.04]} & {\tiny [0.00, 0.24]} & {\tiny [0.19, 1.91]} & {\tiny [0.00, 0.40]} & {\tiny [0.07, 1.04]} & {\tiny [0.00, 0.39]} & {\tiny [0.45, 1.59]} & {\tiny [0.08, 0.65]} & {\tiny [0.15, 0.82]} & {\tiny [0.00, 0.55]} & {\tiny [0.64, 1.97]} & {\tiny [18.47, 24.19]} & {\tiny [17.91, 23.88]} & {\tiny [10.69, 16.35]} & {\tiny [15.32, 20.47]} & \cellcolor{blue!15}{\tiny [33.25, 43.64]} & \cellcolor{red!15}{\tiny [46.28, 56.59]} & \cellcolor{violet!15}{\tiny [28.69, 38.13]} & \cellcolor{orange!15}{\tiny [39.19, 47.26]} & \cellcolor{blue!45}{\tiny [44.03, 55.89]} & \cellcolor{red!45}{\tiny [56.04, 67.01]} & \cellcolor{violet!45}{\tiny [37.50, 49.69]} & \cellcolor{orange!45}{\tiny [55.90, 66.95]} \\
% \cline{1-25}
% pass@5       & 0.41 & 1.79 & 0.39 & 2.65 & 0.48 & 1.20 & 0.47 & 2.73 & 0.97 & 1.34 & 0.71 & 3.40 & 63.51 & 62.12 & 39.81 & 56.29 & \cellcolor{blue!15}72.83 & \cellcolor{red!15}82.43 & \cellcolor{violet!15}61.30 & \cellcolor{orange!15}84.06 & \cellcolor{blue!45}80.21 & \cellcolor{red!45}86.98 & \cellcolor{violet!45}63.13 & \cellcolor{orange!45}86.17 \\
% {\tiny CI} & {\tiny [0.00, 1.21]} & {\tiny [0.37, 3.86]} & {\tiny [0.00, 1.18]} & {\tiny [0.95, 4.96]} & {\tiny [0.00, 1.61]} & {\tiny [0.37, 2.24]} & {\tiny [0.00, 1.18]} & {\tiny [1.59, 4.34]} & {\tiny [0.40, 1.61]} & {\tiny [0.82, 2.24]} & {\tiny [0.39, 1.18]} & {\tiny [1.97, 5.36]} & {\tiny [57.07, 69.75]} & {\tiny [56.04, 67.94]} & {\tiny [33.18, 46.57]} & {\tiny [50.21, 62.30]} & \cellcolor{blue!15}{\tiny [65.79, 79.25]} & \cellcolor{red!15}{\tiny [76.50, 87.95]} & \cellcolor{violet!15}{\tiny [54.32, 68.17]} & \cellcolor{orange!15}{\tiny [78.77, 88.85]} & \cellcolor{blue!45}{\tiny [74.18, 85.70]} & \cellcolor{red!45}{\tiny [81.63, 91.78]} & \cellcolor{violet!45}{\tiny [55.81, 70.04]} & \cellcolor{orange!45}{\tiny [80.64, 91.25]} \\
% \cline{1-25}
% pass@10      & 0.79 & 2.98 & 0.63 & 4.59 & 0.81 & 1.81 & 0.78 & 4.34 & 1.61 & 2.24 & 1.18 & 5.36 & 79.13 & 81.32 & 47.82 & 72.88 & \cellcolor{blue!15}81.50 & \cellcolor{red!15}87.96 & \cellcolor{violet!15}67.21 & \cellcolor{orange!15}89.97 & \cellcolor{blue!45}87.87 & \cellcolor{red!45}91.03 & \cellcolor{violet!45}67.33 & \cellcolor{orange!45}89.65 \\
% {\tiny CI} & {\tiny [0.00, 2.42]} & {\tiny [0.75, 5.97]} & {\tiny [0.00, 1.89]} & {\tiny [1.40, 8.15]} & {\tiny [0.00, 2.02]} & {\tiny [0.75, 3.73]} & {\tiny [0.00, 1.89]} & {\tiny [2.75, 6.97]} & {\tiny [0.40, 3.23]} & {\tiny [0.75, 4.10]} & {\tiny [0.00, 2.75]} & {\tiny [2.75, 8.24]} & {\tiny [71.77, 85.48]} & {\tiny [74.63, 87.31]} & {\tiny [40.25, 55.35]} & {\tiny [65.44, 79.85]} & \cellcolor{blue!15}{\tiny [74.19, 87.90]} & \cellcolor{red!15}{\tiny [82.09, 93.28]} & \cellcolor{violet!15}{\tiny [59.75, 74.21]} & \cellcolor{orange!15}{\tiny [84.59, 94.58]} & \cellcolor{blue!45}{\tiny [81.45, 93.55]} & \cellcolor{red!45}{\tiny [85.82, 95.52]} & \cellcolor{violet!45}{\tiny [59.75, 74.21]} & \cellcolor{orange!45}{\tiny [84.42, 94.45]} \\
% \cline{1-25}
% pass@20      & 0.81 & 2.97 & 0.64 & 5.39 & 1.61 & 2.99 & 1.26 & 7.88 & 3.23 & 4.48 & 1.89 & 9.78 & 79.00 & 81.39 & 47.84 & 75.57 & \cellcolor{blue!15}81.52 & \cellcolor{red!15}88.10 & \cellcolor{violet!15}67.35 & \cellcolor{orange!15}90.79 & \cellcolor{blue!45}87.93 & \cellcolor{red!45}90.99 & \cellcolor{violet!45}67.33 & \cellcolor{orange!45}90.11 \\
% {\tiny CI} & {\tiny [0.00, 2.42]} & {\tiny [0.75, 5.97]} & {\tiny [0.00, 1.89]} & {\tiny [2.29, 9.16]} & {\tiny [0.00, 4.03]} & {\tiny [0.75, 6.45]} & {\tiny [0.00, 3.14]} & {\tiny [4.58, 11.45]} & {\tiny [0.81, 6.45]} & {\tiny [1.49, 8.21]} & {\tiny [0.00, 4.40]} & {\tiny [5.34, 14.50]} & {\tiny [71.77, 85.48]} & {\tiny [74.63, 87.31]} & {\tiny [40.25, 55.35]} & {\tiny [67.94, 83.21]} & \cellcolor{blue!15}{\tiny [74.19, 87.90]} & \cellcolor{red!15}{\tiny [82.09, 93.28]} & \cellcolor{violet!15}{\tiny [59.75, 74.84]} & \cellcolor{orange!15}{\tiny [85.50, 95.42]} & \cellcolor{blue!45}{\tiny [82.26, 93.55]} & \cellcolor{red!45}{\tiny [85.82, 95.52]} & \cellcolor{violet!45}{\tiny [59.75, 74.21]} & \cellcolor{orange!45}{\tiny [84.73, 94.66]} \\
% \cline{1-25}
% AUP@k        & 0.00 & 0.02 & 0.00 & 0.03 & 0.01 & 0.02 & 0.01 & 0.05 & 0.02 & 0.02 & 0.01 & 0.07 & 0.61 & 0.61 & 0.35 & 0.58 & \cellcolor{blue!15}0.70 & \cellcolor{red!15}0.80 & \cellcolor{violet!15}0.57 & \cellcolor{orange!15}0.82 & \cellcolor{blue!45}0.78 & \cellcolor{red!45}0.85 & \cellcolor{violet!45}0.61 & \cellcolor{orange!45}0.85 \\
% {\tiny CI} & {\tiny [0.000, 0.013]} & {\tiny [0.004, 0.039]} & {\tiny [0.000, 0.011]} & {\tiny [0.011, 0.057]} & {\tiny [0.000, 0.022]} & {\tiny [0.004, 0.039]} & {\tiny [0.000, 0.018]} & {\tiny [0.026, 0.084]} & {\tiny [0.004, 0.035]} & {\tiny [0.008, 0.045]} & {\tiny [0.000, 0.025]} & {\tiny [0.036, 0.099]} & {\tiny [0.549, 0.668]} & {\tiny [0.549, 0.658]} & {\tiny [0.294, 0.416]} & {\tiny [0.520, 0.639]} & \cellcolor{blue!15}{\tiny [0.626, 0.765]} & \cellcolor{red!15}{\tiny [0.747, 0.854]} & \cellcolor{violet!15}{\tiny [0.508, 0.637]} & \cellcolor{orange!15}{\tiny [0.770, 0.867]} & \cellcolor{blue!45}{\tiny [0.722, 0.836]} & \cellcolor{red!45}{\tiny [0.800, 0.896]} & \cellcolor{violet!45}{\tiny [0.534, 0.673]} & \cellcolor{orange!45}{\tiny [0.799, 0.901]} \\
% \hline
% \end{longtable}
% \endgroup
% \end{landscape}
